# Supplementary material for: Primordial black hole constraints with Hawking radiation -- a review
Source: arXiv:2206.02672 source file (2022-06-06)
Supplement: Supplementary file 1 [file Appendix.tex]

\section{The Standard Model of particle physics}

The Standard Model of particle physics (SM) is the theory that describes the fundamental particles and their interactions. The idea that the material world can be divided into fundamental indivisible species dates back to Antiquity. However, it is only at the end of the XIX$^e$ century that this theory acquired a predictive power with the discovery of the charged electron. The photon as a carrier of light energy was known for a long time, but its behaviour as a quanta was exposed only with the photoelectric effect. Afterwards, chemistry and nuclear physics experiments have put in evidence the structure of the atom, with a nucleus composed of protons (charged, stable) and neutrons (unstable). The structure of matter revealed itself as the experiments increased in energy, with a collision at energy $E$ probing a fundamental scale of size $L\sim E^{-1}$. Neutrinos were predicted in the 1930's to explain the characteristics of the $\beta$ decays, at the same epoch when the muons (a second family of charged lepton with the electron) were observed in cosmic rays (CRs) and the graviton was predicted to mediate the gravitational interaction. The theory of Maxwell describing the electromagnetic (EM) interactions was quantized in the 1950's in a model called quantum electrodynamics (QED). In the 1960's, the theory of the weak interaction describing the same $\beta$-decay of nuclei gave rise to the Glashow--Weinberg--Salam model of the EW interactions, in the first unification of two fundamental interactions (QED and weak interaction). The development of particle accelerators in the late 1950's--1970's resulted in the production of numerous particles in detectors with a mass spectrum very dense above an energy scale of some hundreds of MeV. To explain this matter of fact, two models were in competition at that time:
\begin{itemize}
    \item the ``Hagedorn model'' that predicted an exponential explosion of the number of dofs above the MeV energy scale~\cite{Hagedorn:346206,1970A&A.....5..184H,Hagedorn:880640};
    \item the ``Gell-Mann model'' that systematically described the observed particle states as a combination of a finite number of 3 flavors of quarks and 8 mediating gluons~\cite{1964PhL.....8..214G}\footnote{See also the reports by Zweig \cite{Zweig:570209}.}, in a theory called quantum chromodynamics (QCD).
\end{itemize}
In the 1960's, the Higgs field was finally proposed to explain the rest masses of particles due to a symmetry spontaneously broken at low energy~\cite{1964PhRvL..13..321E,1964PhRvL..13..508H,1964PhRvL..13..585G}. This was the state of the art in the early 70's, when HR was discovered.

The modern view of the SM of particle physics embeds fundamental particles and gauge bosons to mediate interactions between them:
\begin{itemize}
    \item the charged massive leptons are divided into 3 families: electron, muon, tau and their antiparticles;
    \item the neutrinos of extremely low mass are divided into 3 corresponding families: electron neutrino, muon neutrino and tau neutrino which are Majorana particles;
    \item the massive quarks of the QCD model are divided into 3 families or ``flavors'' with 2 members each: up and down, charm and strange, top and bottom, with their antiparticles;
    \item the 3 interactions are mediated by gauge bosons: the massless photon mediates the EM interaction, the 8 massless gluons mediate the strong interaction, and the massive bosons W$^\pm$ and Z$^0$ mediate the weak interaction;
    \item the massive Higgs boson, which is related to the rest masses of particles by their interaction with the Higgs field;
    \item it is often presumed that their exists a bosonic massless graviton to mediate a quantized version of the gravitational interaction, even if such a theory has not yet been made fully coherent.
\end{itemize}
A summary of the particle properties is given in Table~\ref{tab:particles_1}.

\begin{table}[t]
    \centering
    \begin{tabular*}{0.8\columnwidth}{l@{\extracolsep{\fill}}c@{\extracolsep{\fill}}c@{\extracolsep{\fill}}c@{\extracolsep{\fill}}c}
        \toprule
        particle & symbol & mass (GeV) & spin & internal dofs \\
        \midrule
        Higgs boson	  & $h^0$ & $1.2503\times 10^{2}$  & $0$ & $1$ \\
			photon 		  & $\gamma$  & $0$ 	  & $1$ & $2$ \\
			gluons 		  & $g$ 	  & $0$ 	  & $1$ & $16$ \\
			W bosons	  & $W^\pm$   & $8.0403\times 10^1$  & $1$ & $6$ \\
			Z boson		  & $Z^0$	  & $9.11876\times 10^1$ & $1$ & $3$ \\
			neutrinos	  & $\nu_{e,\mu,\tau},\overline{\nu}_{e,\mu,\tau}$ & $0$ & $\nicefrac{1}{2}$ & $6$ \\
			electron	  & $e^{\pm}$ & $5.109989461\times 10^{-4}$ & $\nicefrac{1}{2}$ & $4$ \\
			muon		  & $\mu^\pm$ & $1.056583745\times 10^{-1}$ & $\nicefrac{1}{2}$ & $4$ \\
			tau			  & $\tau^\pm$ & $1.77686$ & $\nicefrac{1}{2}$ & $4$ \\
			up quark 	  & $u,\overline{u}$ & $2.2\times 10^{-3}$ & $\nicefrac{1}{2}$ & $12$ \\
			down quark 	  & $d,\overline{d}$ & $4.7\times 10^{-3}$ & $\nicefrac{1}{2}$ & $12$ \\
			charm quark   & $c,\overline{c}$ & $1.27$ & $\nicefrac{1}{2}$ & $12$ \\
			strange quark & $s,\overline{s}$ & $9.6\times 10^{-2}$ & $\nicefrac{1}{2}$ & $12$ \\
			top quark 	  & $t,\overline{t}$ & $1.7321\times 10^2$ & $\nicefrac{1}{2}$ & $12$ \\
			bottom quark  & $b,\overline{b}$ & $4.18$ & $\nicefrac{1}{2}$ & $12$ \\
			graviton 	  & $G$ & $0$ & $2$ & $2$ \\
        \bottomrule
    \end{tabular*}
    \caption{Properties of the elementary particles of the Standard Model, in addition to the graviton~\cite{2018PhRvD..98c0001T}. The number of quantum dofs is the product of the family, antiparticle, colour and helicity multiplicities. Neutrinos are here considered massless.}
    \label{tab:particles_1}
\end{table}

The SM is assuredly not the final theory of particle physics, and that for several reasons (this is not a complete list): there is no DM component in this model; the dark energy (cosmological constant?) causing the acceleration of the expansion of the universe is also absent; the neutrinos are proven to be massive by observation of their flavor oscillations; some measurements of particle physics experiments have shown discrepancies with the SM predictions (a famous recent one is the $g-2$ muon magnetic moment); and a renormalizable theory of quantum gravity is still to be found.

Hence, plentiful of models have been proposed to explain the new observational data while safeguarding all the extremely precise SM predictions already confronted to experiments. The most famous is the ``supersymmetric'' model where each particle has a ``superpartner''. These models could embed a quantum theory of gravity (like the ``loop quantum gravity'' or LQG model), and some of them require additional dimensions like string theory. Other DM candidates include axions and right-handed neutrinos. For a complete review and history of those ideas see~\cite{2018RvMP...90d5002B}.

\section{Timelines}

\input{timelines/baryogenesis}

\input{timelines/BBN}

\input{timelines/CMB}

\input{timelines/photons}

\input{timelines/neutrinos}

\input{timelines/electrons}

\input{timelines/final_burst}
